# Supplementary material for: Evaluating List Construction and Temporal Understanding capabilities of Large Language Models
Source: arXiv:2506.21783 source file (2025-06-26)
Supplement: Supplementary file 1 [file appendix.tex]

\newpage

\clearpage

\appendix

%\input{table-datasets}

% \section{Retr}
% \label{sec:datasets}

\begin{figure}
    \centering
    \includegraphics[width=0.9\linewidth]{figures/ndcg_plot.png}
    \caption{Comparison of retrieval models (nDCG) }
                \label{fig:retriever_extra_2}

\end{figure}

\begin{figure}[h]
    \centering
    \includegraphics[width=1\linewidth]{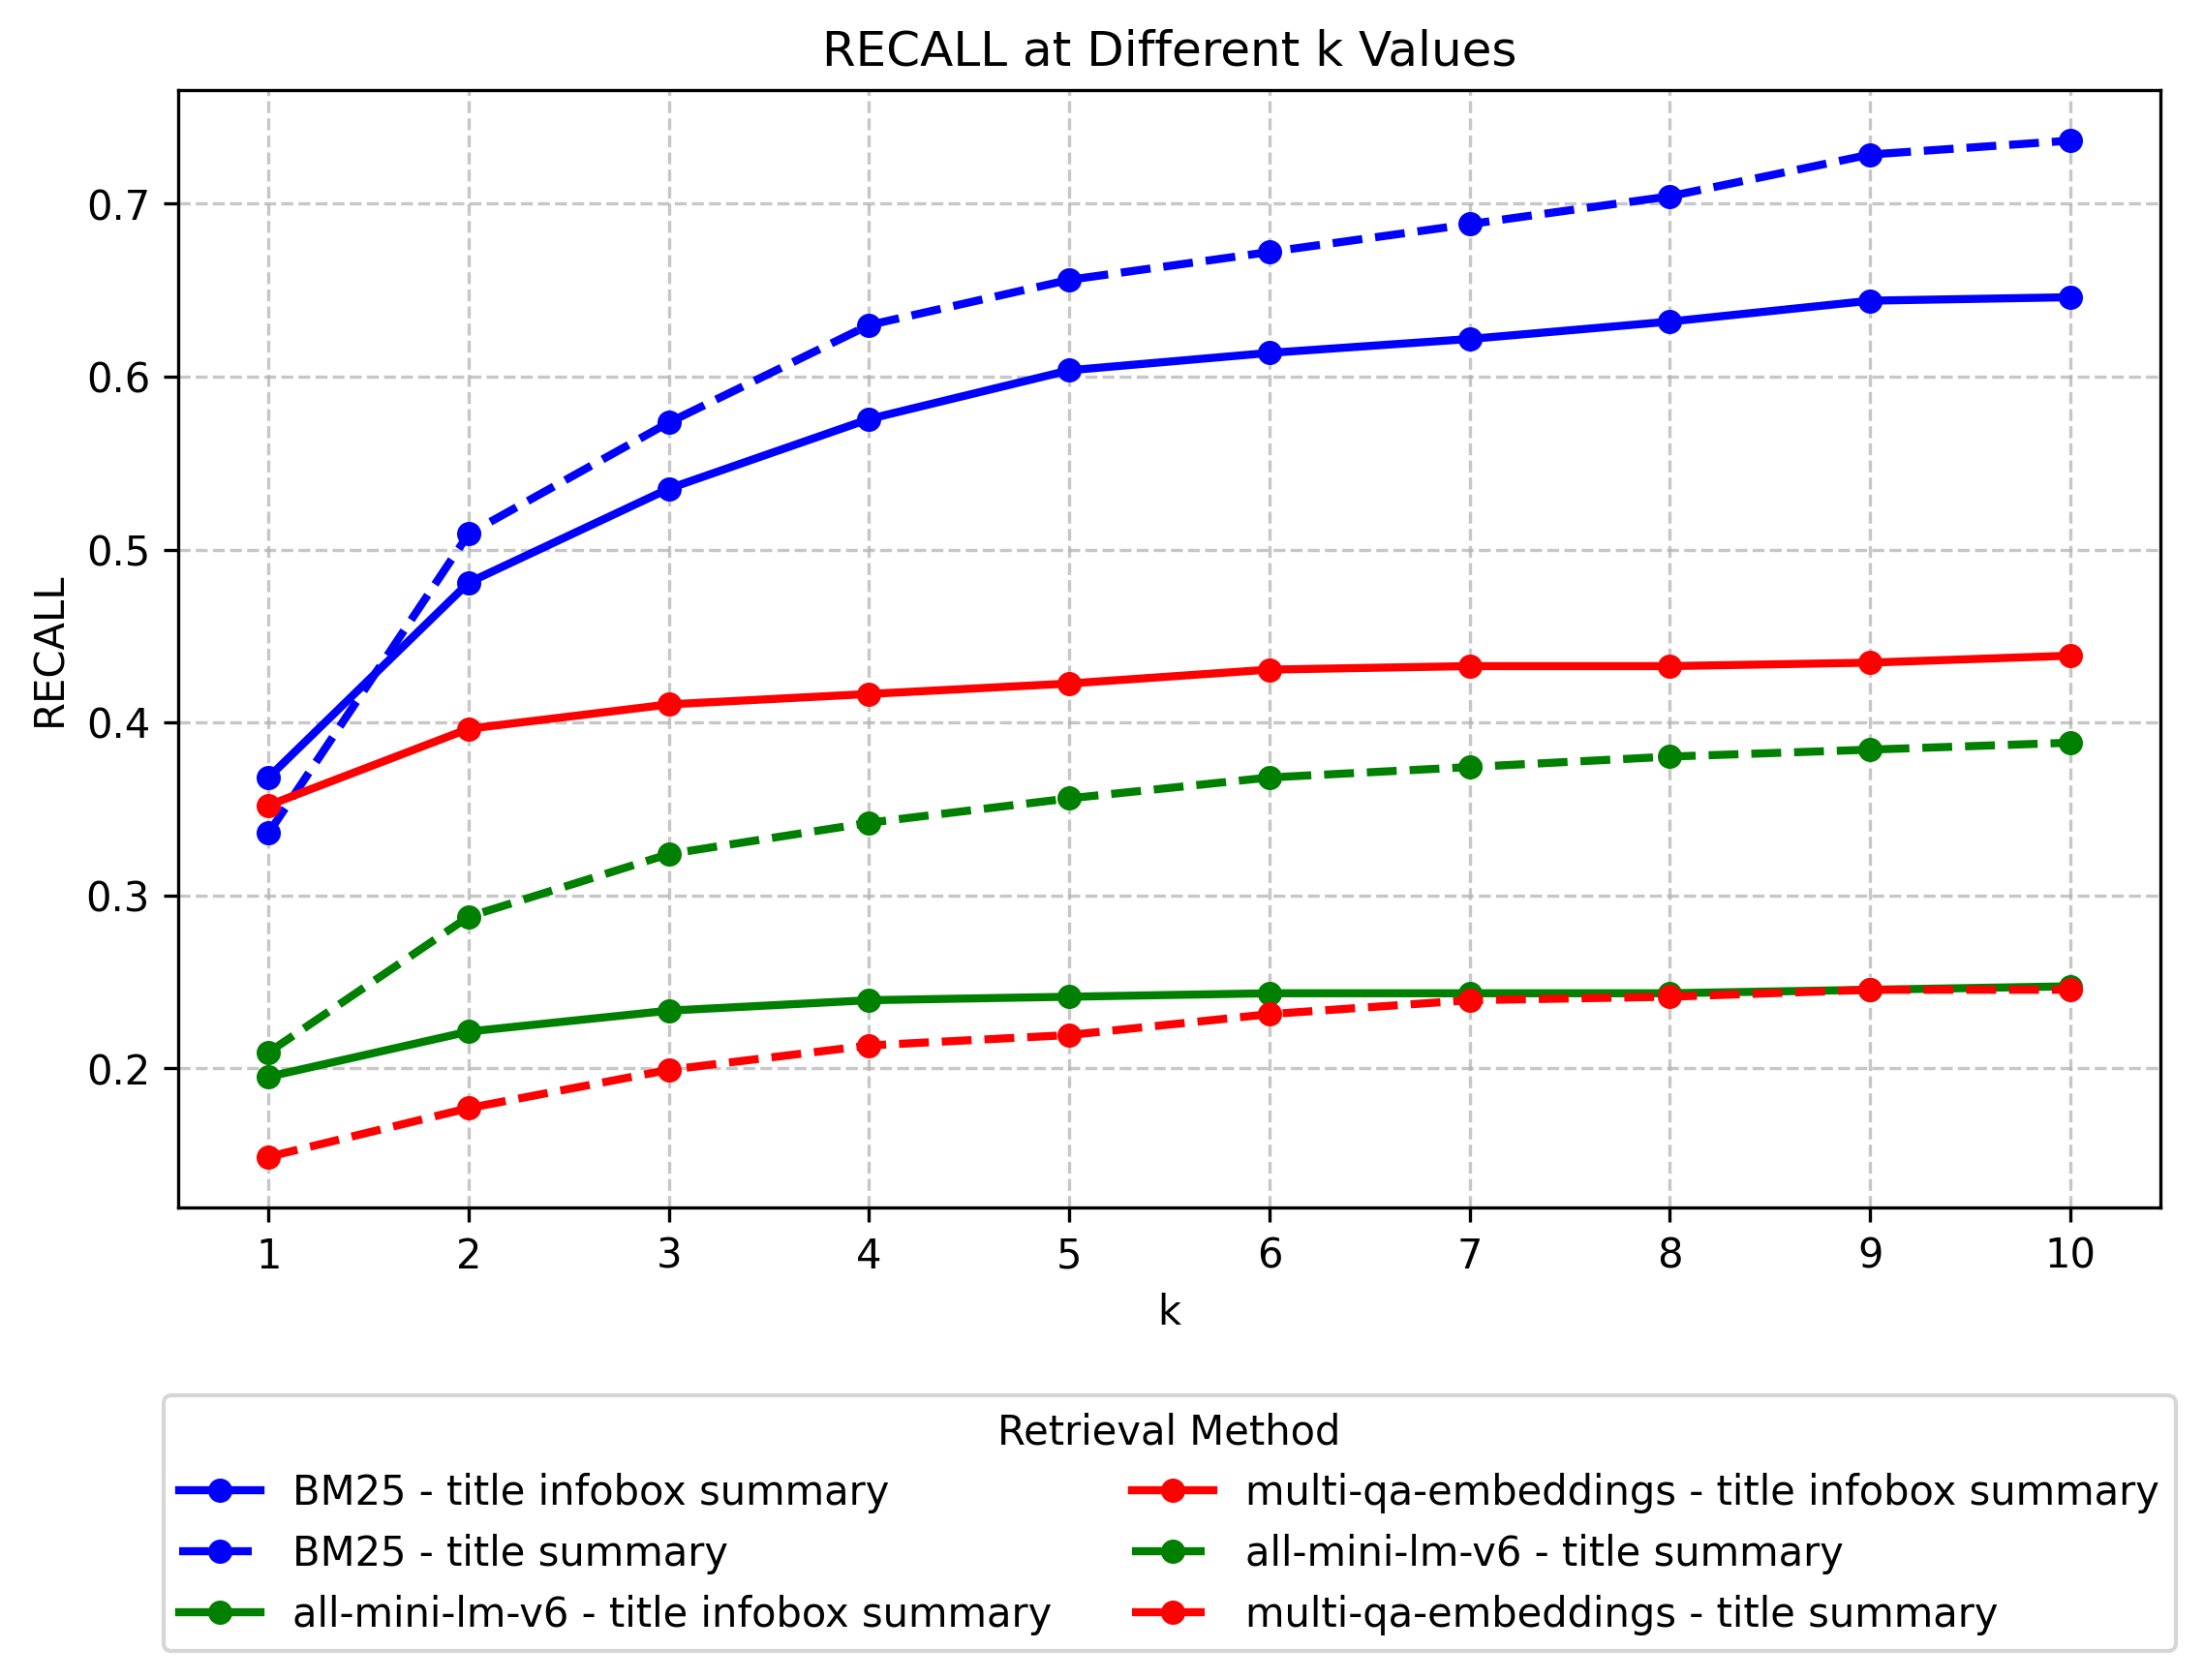}
    \caption{Comparison of retrieval models (Recall) }
                \label{fig:retriever_extra_1}

\end{figure}

\begin{figure}[h]
    \centering
    \includegraphics[width=1\linewidth]{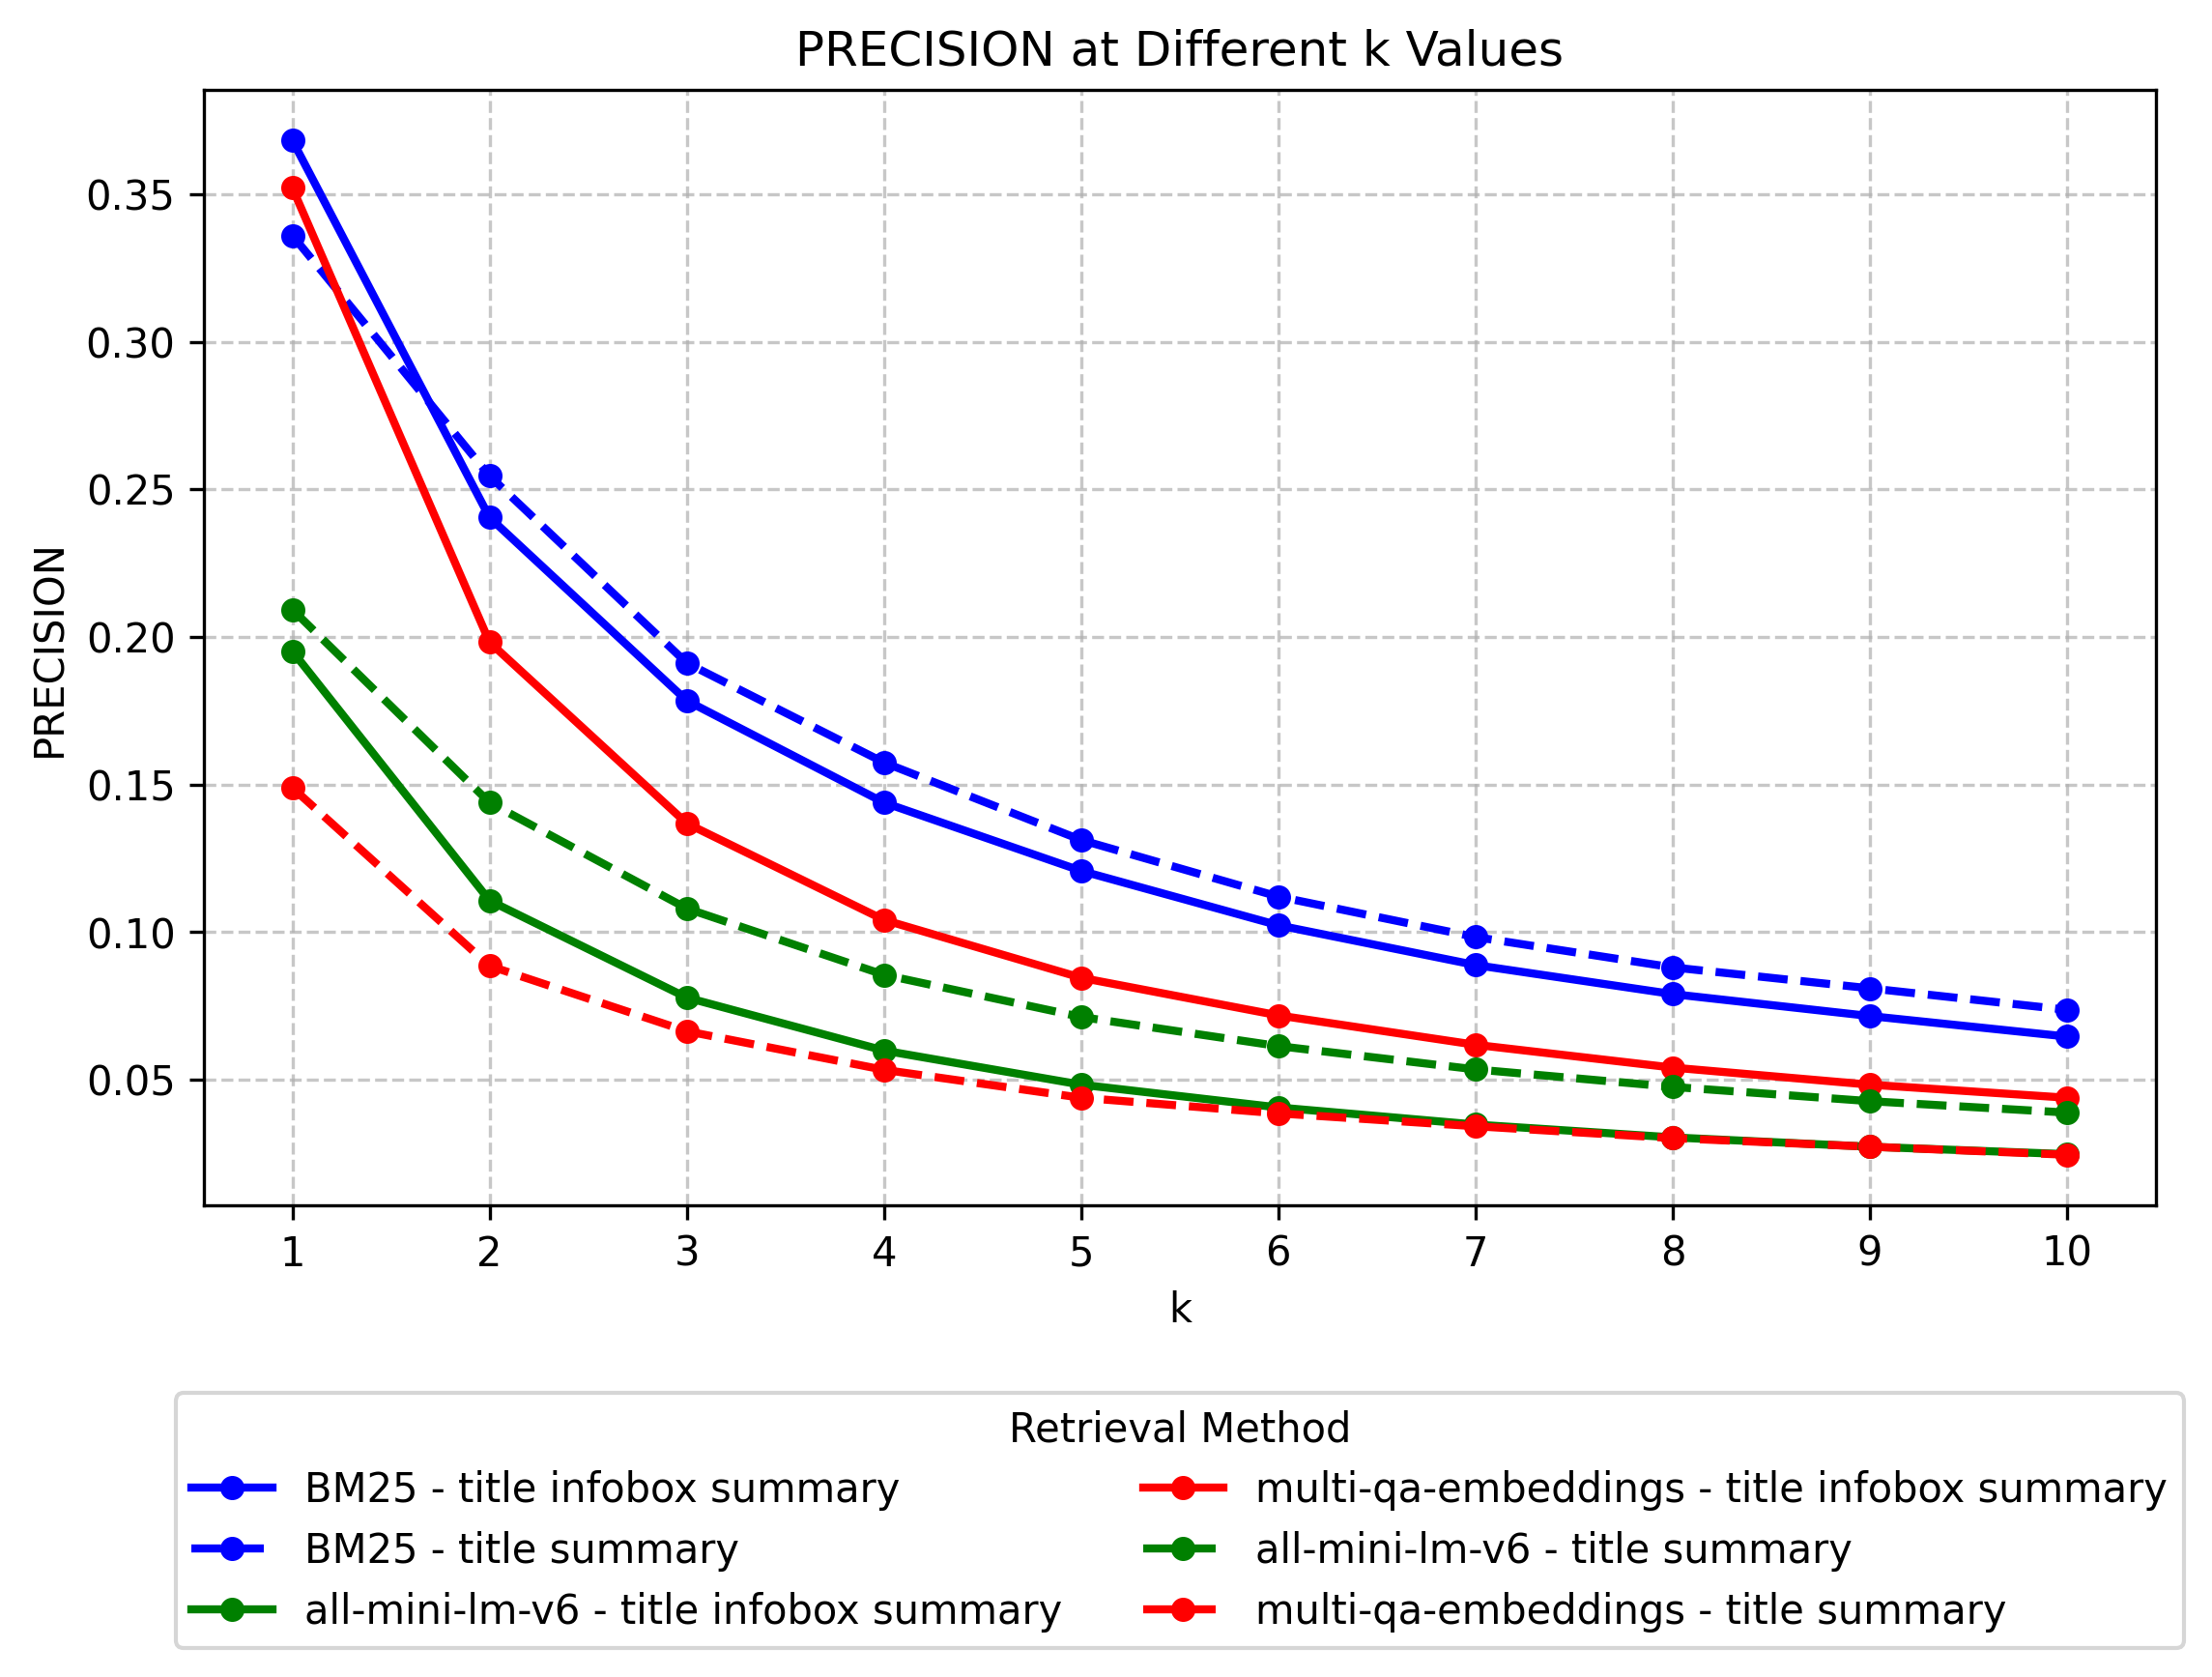}
    \caption{Comparison of retrieval models (Precision). }
        \label{fig:retriever_extra}
\end{figure}
\section{Results using Alternate Open Source LLMs}
\label{sec:small_llms}
